# Supplementary material for: Decentralized Distributed Optimization for Saddle Point Problems
Source: arXiv:2102.07758 source file (2024-04-09)
Supplement: Supplementary file 1 [file appendix_sliding.tex]

\section{Separating the Communication and Oracle Complexities}\label{app:sliding_convergence}

\subsection{Proof of Theorem \ref{Th:distr_MP_sc}}

The proof is analogical to proof of Theorem \ref{Th:distr_MP} presented in Appendix \ref{app:distr_MP}. We let $\mWr = \mWp = \mW$, $\gamma_r = \gamma_p = \gamma$ and consider a regularized function
\begin{align*}
    S_{\alpha}(\xi, \eta) = F(\bx, \bp, \by, \br) + {\gamma}\angles{\bu, \mW\br} + {\gamma}\angles{\bz, \mW\bp} + \frac{\alpha}{2}\norm{\bu}_2^2 - \frac{\alpha}{2}\norm{\bz}_2^2, 
\end{align*}
which is smooth with constant $L_\alpha = \max(L, \gamma\lambda_{\max}(\mW))$ and strongly convex with modulus $\mu_\alpha = \min(\mu, \alpha)$. Analysis of Mirror-Prox in Euclidean strongly-convex-concave case implies that $(m\eps)$-accuracy in $S$ (which corresponds to $\eps$-accuracy in $f$, see end of Appendix \ref{app:distr_MP} for details) is attained after $N = O((L_\alpha / \mu_\alpha) \log(R_\zeta^2 / m\eps))$ iterations. In the case of problem \eqref{eq:problem_reform_regularized}, this complexity takes the form
\begin{align*}
    N 
    &= O\cbraces{\frac{L_\alpha}{\mu_\alpha} \log\cbraces{\frac{R_\zeta^2}{m\eps}}}
    = O\cbraces{\max\cbraces{\frac{L}{\mu}, \frac{\gamma\lambda_{\max}(\mW)}{\mu}, \frac{M^2L}{\gamma\eps\lambda_{\min}^+(\mW)}, \frac{M^2\lambda_{\max}(\mW)}{\eps\lambda_{\min}^+(\mW)}} \cbraces{\frac{R_\zeta^2}{m\eps}}}.
\end{align*}
Taking $\gamma = \frac{L}{\lambda_{\max}(\mW)}$, we balances the terms under $\max$ and finishes the proof.

\subsection{Regularization of Problem \eqref{eq:problem_reform}}\label{app:sliding_regularization}

First, let us show why regularization of a saddle-point problem is valid, i.e. why solutions of \eqref{eq:problem_reform_regularized} and \eqref{eq:problem_reform} are close enough. We use denotations of Appendix \ref{app:mp_smoothness_constants}, i.e. groups of variables $\xi=(\bx^\top,\bp^\top,\bu^\top)^\top$, $\eta=(\by^\top,\br^\top,\bz^\top)^\top$ and 
\[
S(\xi,\eta) =   F(\bx, \bp, \by, \br) + {\gamma_r}\angles{\bu, \mWr\br} + {\gamma_p}\angles{\bz, \mWp\bp}.
\]
We denote the regularized variant of $S$ as
\begin{align*}
    S_{\alpha}(\xi, \eta) = F(\bx, \bp, \by, \br) + {\gamma_r}\angles{\bu, \mWr\br} + {\gamma_p}\angles{\bz, \mWp\bp} + \frac{\alpha}{2}\norm{\bu}_2^2 - \frac{\alpha}{2}\norm{\bz}_2^2,
\end{align*}
where 
$$
\alpha = \frac{\eps\min(\gamma_p\lambda_{\min}^+(\mWp), \gamma_r\lambda_{\min}^+(\mWr))}{8mM^2}.
$$

\begin{lemma}
    Let $(\hat\xi, \hat\eta)$ be a $(\eps/2)$-solution of regularized problem \eqref{eq:problem_reform_regularized}, i.e. it holds
    \begin{align*}
        \max_{\eta\in C_\eta} S_\alpha(\hat\xi, \eta) - \min_{\xi\in C_\xi} S_\alpha(\xi, \hat\eta) \leq \frac{\eps}{2}.
    \end{align*}
    Then $(\hat\xi, \hat\eta)$ is an $\eps$-solution of non-regularized problem \eqref{eq:problem_reform_constrained}, i.e.
    \begin{align*}
        \max_{\eta\in C_\eta} S(\hat\xi, \eta) - \min_{\xi\in C_\xi} S(\xi, \hat\eta) \leq \eps.
    \end{align*}
\end{lemma}

\begin{proof}
    Define $\ds\tilde\eta = \argmax_{\eta\in C_\eta} S(\hat\xi, \eta)$ and $\ds\tilde\xi = \argmin_{\xi\in C_\xi} S(\xi, \hat\eta)$. It holds
    \begin{align*}
        \max_{\eta\in Q_\eta} S_\alpha(\hat\xi, \eta) 
        &= \max_{\eta\in Q_\eta}\sbraces{S(\hat\xi, \eta) + \frac{\alpha}{2}\norm{\hat\bu}_2^2 - \frac{\alpha}{2}\norm{\bz}_2^2} 
        \geq S(\hat\xi, \tilde\eta) + \frac{\alpha}{2}\norm{\hat\bu}_2^2 - \frac{\alpha}{2}\norm{\tilde\bz}_2^2 \\ 
        &\geq \max_{\eta\in C_\eta} S(\hat\xi, \eta) - \frac{\alpha}{2} R_z^2
        \geq \max_{\eta\in C_\eta} S(\hat\xi, \eta) - \frac{\eps}{4}.
    \end{align*}
    Analogously, 
    \begin{align*}
        \min_{\xi\in Q_\xi} S_\alpha(\xi, \hat\eta)
        &= \min_{\xi\in Q_\xi} \sbraces{S(\xi, \hat\eta) + \frac{\alpha}{2}\norm{\bu}_2^2 - \frac{\alpha}{2}\norm{\hat\bz}_2^2}
        \leq S(\tilde\xi, \hat\xi) + \frac{\alpha}{2}\norm{\tilde\bu}_2^2 - \frac{\alpha}{2}\norm{\hat\bz}_2^2 \\
        &\leq \min_{\xi\in C_\xi} S(\xi, \hat\eta) + \frac{\alpha}{2} R_u^2
        \leq \min_{\xi\in C_\xi} S(\xi, \hat\eta) + \frac{\eps}{4}.
    \end{align*}
    Therefore, we obtain
    \begin{align*}
        \max_{\eta\in C_\eta} S(\hat\xi, \eta) - \min_{\xi\in C_\xi} S(\xi, \hat\eta) \leq 
        \max_{\eta\in C_\eta} S_\alpha(\hat\xi, \eta) - \min_{\xi\in C_\xi} S_\alpha(\xi, \hat\eta) + \frac{\eps}{2} \leq \eps.
    \end{align*}
\end{proof}

\subsection{Convergence Proof for Sliding}\label{app:sliding_theorem_proof}

\begin{lemma}
	Iterates of Algorithm~\ref{alg:sliding} satisfy the following inequality:
	\begin{align}
		\sqn{\zeta^{k+1} - \zeta^*}
		&\leq (1-\eta\mu_g)\sqn{\zeta^k - \zeta^*}+ \left(3\eta\mu_g + \eta^2L_A^2 -  1\right)\sqn{\zeta^k - \theta^k} \notag \\
		&\quad+ \left(\frac{4}{\eta\mu_g} + \frac{4\eta L_B^2}{\mu_g}\right) \sqn{\theta^k - \hat{\theta}^k}. \label{sliding:eq:1}
	\end{align}
\end{lemma}
\begin{proof}
    % could not fix troubles with algorithm line cross reference
    % doing it manually
    % sliding:line:z -> 2
    % sliding:line:y -> 3
    % sliding:line:w -> 4
    % sliding:line:x -> 5
	We start with using line 5 %\ref{sliding:line:x} 
	of Algorithm~\ref{alg:sliding}:
	\begin{align*}
		\sqn{\zeta^{k+1} - \zeta^*}
		&=
		\sqn{\proj_Q(\omega^k) - \proj_Q(\zeta^*)}
		\\&\leq
		\sqn{\omega^k - \zeta^*}.
		\\&=
		\sqn{\zeta^k - \zeta^*} + 2\<\omega^k - \zeta^k, \zeta^k - \zeta^*> + \sqn{\omega^k - \zeta^k}
		\\&=
		\sqn{\zeta^k - \zeta^*} + 2\<\omega^k - \zeta^k, \theta^k - \zeta^*>  + 2\<\omega^k - \zeta^k,\zeta^k - \theta^k> + \sqn{\omega^k - \zeta^k}
		\\&=
		\sqn{\zeta^k - \zeta^*} + 2\<\omega^k - \zeta^k, \theta^k - \zeta^*>  + \sqn{\omega^k - \theta^k} - \sqn{\zeta^k - \theta^k}.
	\end{align*}
	Using line 4 %\ref{sliding:line:w}
	of Algorithm~\ref{alg:sliding} we get
	\begin{align*}
		\sqn{\zeta^{k+1} - \zeta^*}
		&\leq
		\sqn{\zeta^k - \zeta^*} + 2\<\theta^k + \eta(A(\zeta^k) - A(\theta^k)) - \zeta^k, \theta^k - \zeta^*> \\
		&\quad+ \sqn{\omega^k - \theta^k} - \sqn{\zeta^k - \theta^k} \\
		&= \sqn{\zeta^k - \zeta^*} + 2\<\theta^k + \eta A(\zeta^k) - \zeta^k, \theta^k - \zeta^*>-2\eta\<A(\theta^k), \theta^k - \zeta^*> \\
		&\quad+ \sqn{\omega^k - \theta^k} - \sqn{\zeta^k - \theta^k}
	\end{align*}
	Using line 2 %\ref{sliding:line:z}
	of Algorithm~\ref{alg:sliding} we get
	\begin{align*}
	\sqn{\zeta^{k+1} - \zeta^*}
	&\leq
	\sqn{\zeta^k - \zeta^*} + 2\<\theta^k - \nu^k, \theta^k - \zeta^*>  - 2\eta\<A(\theta^k), \theta^k - \zeta^*> + \sqn{\omega^k - \theta^k} - \sqn{\zeta^k - \theta^k}
	\\&=
	\sqn{\zeta^k - \zeta^*} - 2\<\hat{\theta}^k - \nu^k, \zeta^* - \theta^k>  - 2\eta\<A(\theta^k), \theta^k - \zeta^*> + \sqn{\omega^k - \theta^k} - \sqn{\zeta^k - \theta^k}
	\\&\quad+
	2\<\theta^k - \hat{\theta}^k,\theta^k - \zeta^*>.
	\end{align*}
	Using \eqref{sliding:eq:prox} we get
	\begin{align*}
	\sqn{\zeta^{k+1} - \zeta^*}
	&\leq
	\sqn{\zeta^k - \zeta^*} + 2\eta\<B(\hat{\theta}^k), \zeta^* - \theta^k>  - 2\eta\<A(\theta^k), \theta^k - \zeta^*> + \sqn{\omega^k - \theta^k} - \sqn{\zeta^k - \theta^k}
	\\&\quad+
	2\<\theta^k - \hat{\theta}^k,\theta^k - \zeta^*>
	\\&=
	\sqn{\zeta^k - \zeta^*} - 2\eta\<B(\theta^k), \theta^k - \zeta^* >  - 2\eta\<A(\theta^k), \theta^k - \zeta^*> + \sqn{\omega^k - \theta^k} - \sqn{\zeta^k - \theta^k}
	\\&\quad+
	2\<\theta^k - \hat{\theta}^k + \eta (B(\theta^k) - B(\hat{\theta}^k)),\theta^k - \zeta^*>.
	\end{align*}
	Using that $g(\zeta) = A(\zeta) + B(\zeta)$ and $\mu_g$-strong monotonicity of $g$ we get
	\begin{align*}
		\sqn{\zeta^{k+1} - \zeta^*}
		&\leq
		\sqn{\zeta^k - \zeta^*} - 2\eta\<g(\theta^k), \theta^k - \zeta^* >  +\sqn{\omega^k - \theta^k} - \sqn{\zeta^k - \theta^k}
		\\&\quad+
		2\<\theta^k - \hat{\theta}^k + \eta (B(\theta^k) - B(\hat{\theta}^k)),\theta^k - \zeta^*>
		\\&\leq
		\sqn{\zeta^k - \zeta^*}- 2\eta\mu_g\sqn{\theta^k - \zeta^*} - 2\eta\<g(\zeta^*), \theta^k - \zeta^* >  +\sqn{\omega^k - \theta^k} - \sqn{\zeta^k - \theta^k}
		\\&\quad+
		2\<\theta^k - \hat{\theta}^k + \eta (B(\theta^k) - B(\hat{\theta}^k)),\theta^k - \zeta^*>.
	\end{align*}
	By definition of $\zeta^*$ and Young's inequality we get
	\begin{align*}
		\sqn{\zeta^{k+1} - \zeta^*}
		&\leq
		\sqn{\zeta^k - \zeta^*}- 2\eta\mu_g\sqn{\theta^k - \zeta^*}+\sqn{\omega^k - \theta^k} - \sqn{\zeta^k - \theta^k}
		\\&\quad+
		2\<\theta^k - \hat{\theta}^k + \eta (B(\theta^k) - B(\hat{\theta}^k)),\theta^k - \zeta^*>
		\\&\leq
		\sqn{\zeta^k - \zeta^*}- 2\eta\mu_g\sqn{\theta^k - \zeta^*}+\sqn{\omega^k - \theta^k} - \sqn{\zeta^k - \theta^k}
		\\&\quad+
		\frac{\eta\mu_g}{2}\sqn{\theta^k - \zeta^*} + \frac{2}{\eta\mu_g}\sqn{\theta^k - \hat{\theta}^k + \eta (B(\theta^k) - B(\hat{\theta}^k))}
		\\&\leq
		\sqn{\zeta^k - \zeta^*}- \frac{3\eta\mu_g}{2}\sqn{\theta^k - \zeta^*}+\sqn{\omega^k - \theta^k} - \sqn{\zeta^k - \theta^k}
		\\&\quad+
		\frac{4}{\eta\mu_g}\sqn{\theta^k - \hat{\theta}^k} + \frac{4\eta}{\mu_g}\sqn{B(\theta^k) - B(\hat{\theta}^k)}.
	\end{align*}
	Using line 4 %\ref{sliding:line:w}
	of Algorithm~\ref{alg:sliding} we get
	\begin{align*}
		\sqn{\zeta^{k+1} - \zeta^*}
		&\leq
		\sqn{\zeta^k - \zeta^*}- \frac{3\eta\mu_g}{2}\sqn{\theta^k - \zeta^*}+ \eta^2\sqn{A(\zeta^k) - A(\theta^k)} - \sqn{\zeta^k - \theta^k}
		\\&\quad+
		\frac{4}{\eta\mu_g}\sqn{\theta^k - \hat{\theta}^k} + \frac{4\eta}{\mu_g}\sqn{B(\theta^k) - B(\hat{\theta}^k)}.
	\end{align*}
	Using \eqref{eq:LA} and \eqref{eq:LB} we get
	\begin{align*}
	\sqn{\zeta^{k+1} - \zeta^*}
	&\leq
	\sqn{\zeta^k - \zeta^*}- \frac{3\eta\mu_g}{2}\sqn{\theta^k - \zeta^*}+ \eta^2L_A^2\sqn{\zeta^k - \theta^k} - \sqn{\zeta^k - \theta^k}
	\\&\quad+
	\frac{4}{\eta\mu_g}\sqn{\theta^k - \hat{\theta}^k} + \frac{4\eta L_B^2}{\mu_g}\sqn{\theta^k - \hat{\theta}^k}.
	\end{align*}
	Using inequality $\sqn{a+b} \geq \frac{2}{3}\sqn{a} - 2\sqn{b}$ we get
	\begin{align*}
	\sqn{\zeta^{k+1} - \zeta^*}
	&\leq
	\sqn{\zeta^k - \zeta^*}- \frac{3\eta\mu_g}{2}\left[\frac{2}{3}\sqn{\zeta^k - \zeta^*} - 2\sqn{\zeta^k - \theta^k}\right]+ \eta^2L_A^2\sqn{\zeta^k - \theta^k} 
	\\&\quad- \sqn{\zeta^k - \theta^k}+
	\frac{4}{\eta\mu_g}\sqn{\theta^k - \hat{\theta}^k} + \frac{4\eta L_B^2}{\mu_g}\sqn{\theta^k - \hat{\theta}^k}
	\\&\leq
	(1-\eta\mu_g)\sqn{\zeta^k - \zeta^*}+ 3\eta\mu_g\sqn{\zeta^k - \theta^k} + \eta^2L_A^2\sqn{\zeta^k - \theta^k} - \sqn{\zeta^k - \theta^k}
	\\&\quad+
	\frac{4}{\eta\mu_g}\sqn{\theta^k - \hat{\theta}^k} + \frac{4\eta L_B^2}{\mu_g}\sqn{\theta^k - \hat{\theta}^k}
	\\&=
	(1-\eta\mu_g)\sqn{\zeta^k - \zeta^*}+ \left(3\eta\mu_g + \eta^2L_A^2 -  1\right)\sqn{\zeta^k - \theta^k}
	\\&\quad+ 
	\left(\frac{4}{\eta\mu_g} + \frac{4\eta L_B^2}{\mu_g}\right) \sqn{\theta^k - \hat{\theta}^k}.
	\end{align*}
\end{proof}

\begin{lemma}
	Let $\theta^k$ be the output of Forward-Backward-Forward algorithm for solving auxiliary problem \eqref{sliding:eq:prox} after $T$ iterations starting at point $\zeta^k$. Choosing $\delta \in (0, 1/4]$ and number of iterations
	\begin{equation}\label{sliding:eq:T}
		T = \cO \left( \left(1 + \eta L_B\right) \log \frac{1}{\delta}\right)
	\end{equation}
	implies
	\begin{equation}\label{sliding:eq:2}
		\sqn{\hat{\theta}^k - \theta^k} \leq 4\delta\sqn{\zeta^k - \theta^k}.
	\end{equation}
\end{lemma}
\begin{proof}
	Problem \eqref{sliding:eq:prox} is a variational inequality of the form
	\begin{equation*}
		\<\hat{B}^k(\hat{\theta}^k), \zeta - \hat{\theta}^k> \geq 0 \text{ for all } \zeta \in Q,
	\end{equation*}
	where operator $\hat{B}^k \colon Q \rightarrow \R^d$ is defined in the following way
	\begin{equation*}
		\hat{B}^k(\zeta) = \eta B(\zeta) + \zeta - \nu^k.
	\end{equation*}
	Operator $\hat{B}^k(\zeta)$ is 1-strongly monotone and $(1 + \eta L_B)$-Lipschitz. Hence, applying the standard result on Forward-Backward-Forward algorithm implies
	\begin{equation*}
		\sqn{\theta^k - \hat{\theta}^k} \leq \delta\sqn{\zeta^k - \hat{\theta}^k}.
	\end{equation*}
	Moreover,
	\begin{align*}
		\sqn{\theta^k - \hat{\theta}^k} &\leq \delta\sqn{\zeta^k - \hat{\theta}^k}
		\\&\leq
		2\delta\sqn{\zeta^k - \theta^k} + 2\delta\sqn{\theta^k - \hat{\theta}^k}
		\\&\leq
		2\delta\sqn{\zeta^k - \theta^k} + \frac{1}{2}\sqn{\theta^k - \hat{\theta}^k},
	\end{align*}
	where the last inequality follows from $\delta \leq \frac{1}{4}$. Rearranging gives \eqref{sliding:eq:2}.
\end{proof}

\begin{lemma}
 Apply Algorithm~\ref{alg:sliding} to the problem \eqref{eq:problem_reform}. On each iteration of Algorithm~\ref{alg:sliding} solve auxiliary problem \eqref{sliding:eq:prox} on line 3 %\ref{sliding:line:y}
 with $T$ iterations of Forward-Backward-Forward algorithm starting at point $\zeta^k$, where $T$ is given by \eqref{sliding:eq:T}
 Choosing $\delta$ to be
 \begin{equation}\label{sliding:delta}
 	\delta = \min\left\{\frac{1}{4}, \left[\frac{64}{\eta\mu_g} + \frac{64\eta L_B^2}{\mu_g}\right]^{-1}\right\},
 \end{equation}
 choosing stepsize $\eta$ to be
 \begin{equation}\label{sliding:eta}
 	\eta = \min\left\{\frac{1}{2L_A}, \frac{1}{6\mu_g}\right\}
 \end{equation}
 and choosing number of iterations $N$ to be
 \begin{equation}\label{sliding:K}
 	N = \frac{1}{\eta\mu_g} \log \frac{\sqn{\zeta^0 - \zeta^*}}{\epsilon}
 \end{equation}
 implies
 \begin{equation}\label{sliding:eq:3}
 	\sqn{\zeta^N - \zeta^*} \leq \epsilon.
 \end{equation}
\end{lemma}
\begin{proof}
	Using \eqref{sliding:eq:1} together with \eqref{sliding:eq:2}, we get
	\begin{align*}
		\sqn{\zeta^{k+1} - \zeta^*}
		&\leq (1-\eta\mu_g)\sqn{\zeta^k - \zeta^*}+ \left(3\eta\mu_g + \eta^2L_A^2 -  1\right)\sqn{\zeta^k - \theta^k}
		\\
		&\quad+ 4\delta\left(\frac{4}{\eta\mu_g} + \frac{4\eta L_B^2}{\mu_g}\right) \sqn{\zeta^k - \theta^k}.
	\end{align*}
	Plugging $\delta$ defined by \eqref{sliding:delta} gives
	\begin{align*}
	\sqn{\zeta^{k+1} - \zeta^*}&\leq (1-\eta\mu_g)\sqn{\zeta^k - \zeta^*}+ \left(3\eta\mu_g + \eta^2L_A^2 -  1\right)\sqn{\zeta^k - \theta^k}
	+
	\frac{1}{4}\sqn{\zeta^k - \theta^k}
	\\&=
	(1-\eta\mu_g)\sqn{\zeta^k - \zeta^*}+ \left(3\eta\mu_g + \eta^2L_A^2 -  \frac{3}{4}\right)\sqn{\zeta^k - \theta^k}.
	\end{align*}
	Plugging $\eta$ defined by \eqref{sliding:eta} gives
	\begin{align*}
	\sqn{\zeta^{k+1} - \zeta^*}\leq
	(1-\eta\mu_g)\sqn{\zeta^k - \zeta^*}.
	\end{align*}
	After telescoping and using $N$ defined by $\eqref{sliding:K}$ we get \eqref{sliding:eq:3}, which concludes the proof.
\end{proof}

\begin{corollary}
	Without loss of generality assume $L_A \leq L_B$. Total number of computations of $A(\zeta)$ is
	\begin{equation*}
		N_A = N = \cO\left(\left(1 + \frac{L_A}{\mu_g}\right)\log \frac{\sqn{\zeta^0 - \zeta^*}}{\epsilon}\right).
	\end{equation*}
	Total number of computations of $B(\zeta)$ is
	\begin{align*}
		N_B &= N \times T= \cO\left(\left(1 + \min\left\{\frac{1}{\mu_g}, \frac{1}{L_A}\right\}L_B\right)\left(1 + \frac{L_A}{\mu_g}\right)\log\frac{1}{\delta}\log \frac{\sqn{\zeta^0 - \zeta^*}}{\epsilon}\right)
		\\&=
		\cO\left(\left(
		1 + \min\left\{\frac{L_B}{\mu_g}, \frac{L_B}{L_A}\right\} + \frac{L_A}{\mu_g} + \min\left\{\frac{L_BL_A}{\mu_g^2}, \frac{L_B}{\mu_g}\right\}
		\right)\log\frac{1}{\delta}\log \frac{\sqn{\zeta^0 - \zeta^*}}{\epsilon}\right)
		\\&\leq
		\cO\left(\left(
		1 + \frac{L_A}{\mu_g}+ \frac{L_B}{\mu_g}
		\right)\log\frac{1}{\delta}\log \frac{\sqn{\zeta^0 - \zeta^*}}{\epsilon}\right)
		\\&\leq
		\cO\left(\left(
		1 +\frac{L_B}{\mu_g}
		\right)\log\frac{1}{\delta}\log \frac{\sqn{\zeta^0 - \zeta^*}}{\epsilon}\right).
	\end{align*}
\end{corollary}
